# Supplementary material for: Magic123: One Image to High-Quality 3D Object Generation Using Both 2D and 3D Diffusion Priors
Source: arXiv:2306.17843 source file (2023-07-23)
Supplement: Supplementary file 1 [file supplement.tex]

%%%%%%%%% TITLE
% \clearpage
% \title{PointNeXt: Revisiting PointNet++ with Improved Training and Scaling Strategies \\ 
% --- Supplementary Material ---
% }
% \author{}
% \maketitle
% \begin{center}
% {\large\bf Magic123: One Image to High-Quality 3D Object Generation Using Both 2D and 3D Diffusion Priors
% }\\
% \vspace{1em}
% {\large\bf--- Supplementary Material ---}
% \end{center}

\setcounter{section}{0}
\setcounter{table}{0}
\setcounter{figure}{0}

In this appendix, we provide additional content to complement the main manuscript:
\begin{itemize}[leftmargin=1em,topsep=0pt]

\item Dataset details;

\item Quantitative comparison with the state-of-the-art;

\item Additional qualitative comparison with more prior works including Point-E \cite{PointE}, Shap-E \cite{ShapeE}, and RealFusion \cite{RealFusion}. 

\item Ablation and analysis on the usage of both 2D and 3D priors;

% \item Ablation and analysis on the two-stage optimization; 

% \item Ablation and analysis on textural inversion; 

\end{itemize}

% \item Maximum resolution in both stages and the ideal resolution for each case to enable the best performance.

\section{Dataset details}\label{sec:dataset}

\inlinesection{RealFusion15} We use the dataset collected and released by RealFusion \cite{RealFusion}, consisting of 15 natural images including bananas, birds, cacti, barbie cakes, cat statues, teapots, microphones, dragon statues, fishes, cherries, and watercolor paintings \etc. Among them, watercolor paintings and statues are uncommon objects, while the others are common.
We name this dataset RealFusion15 and show it 
in \figlabel~\ref{fig:realfusion15_dataset}. 

\begin{figure}[h]
\centering
\includegraphics[width=0.9\textwidth]{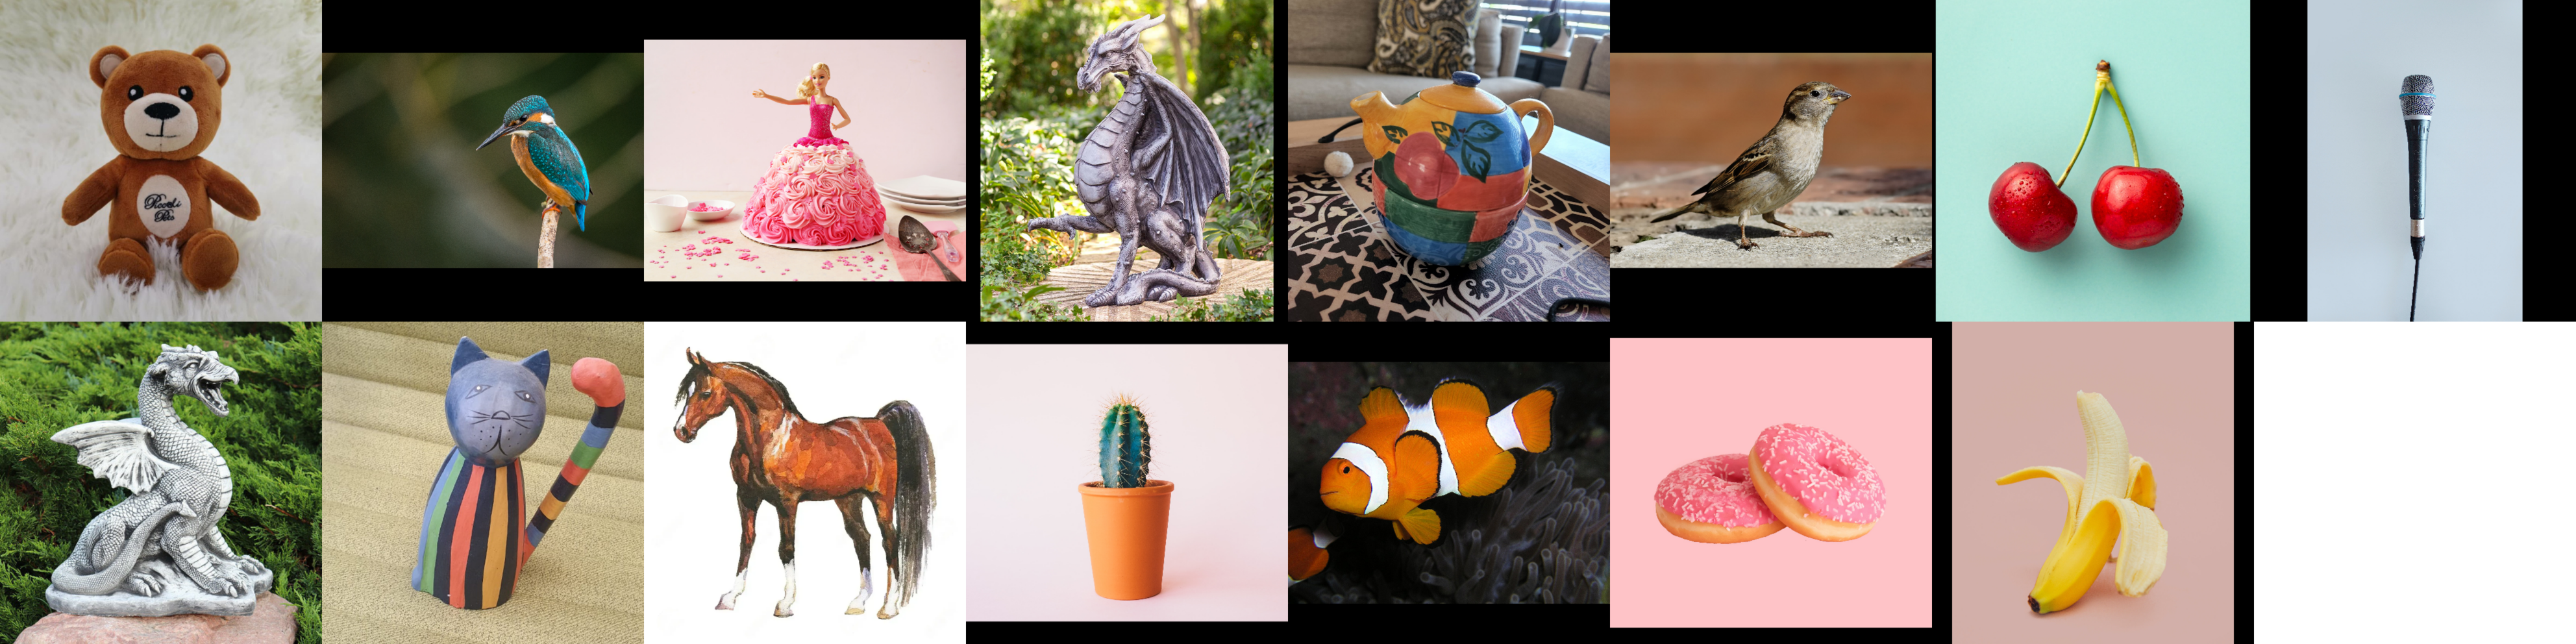}
\caption{Input images from RealFusion15 dataset.}
\label{fig:realfusion15_dataset}
\end{figure}

\inlinesection{NeRF4} 
We additionally introduce a NeRF4 (\figlabel~\ref{fig:nerf4_dataset}) dataset that we collect from 4 scenarios, chair, drums, ficus, and microphone, out of the 8 test examples from the synthetic NeRF dataset. 
These four scenarios are selected to cover complex objects (drums and ficus), a hard case (the back view of the chair), and a simple case (the microphone). 

\begin{figure}[h]
\centering
\includegraphics[width=0.8\textwidth]{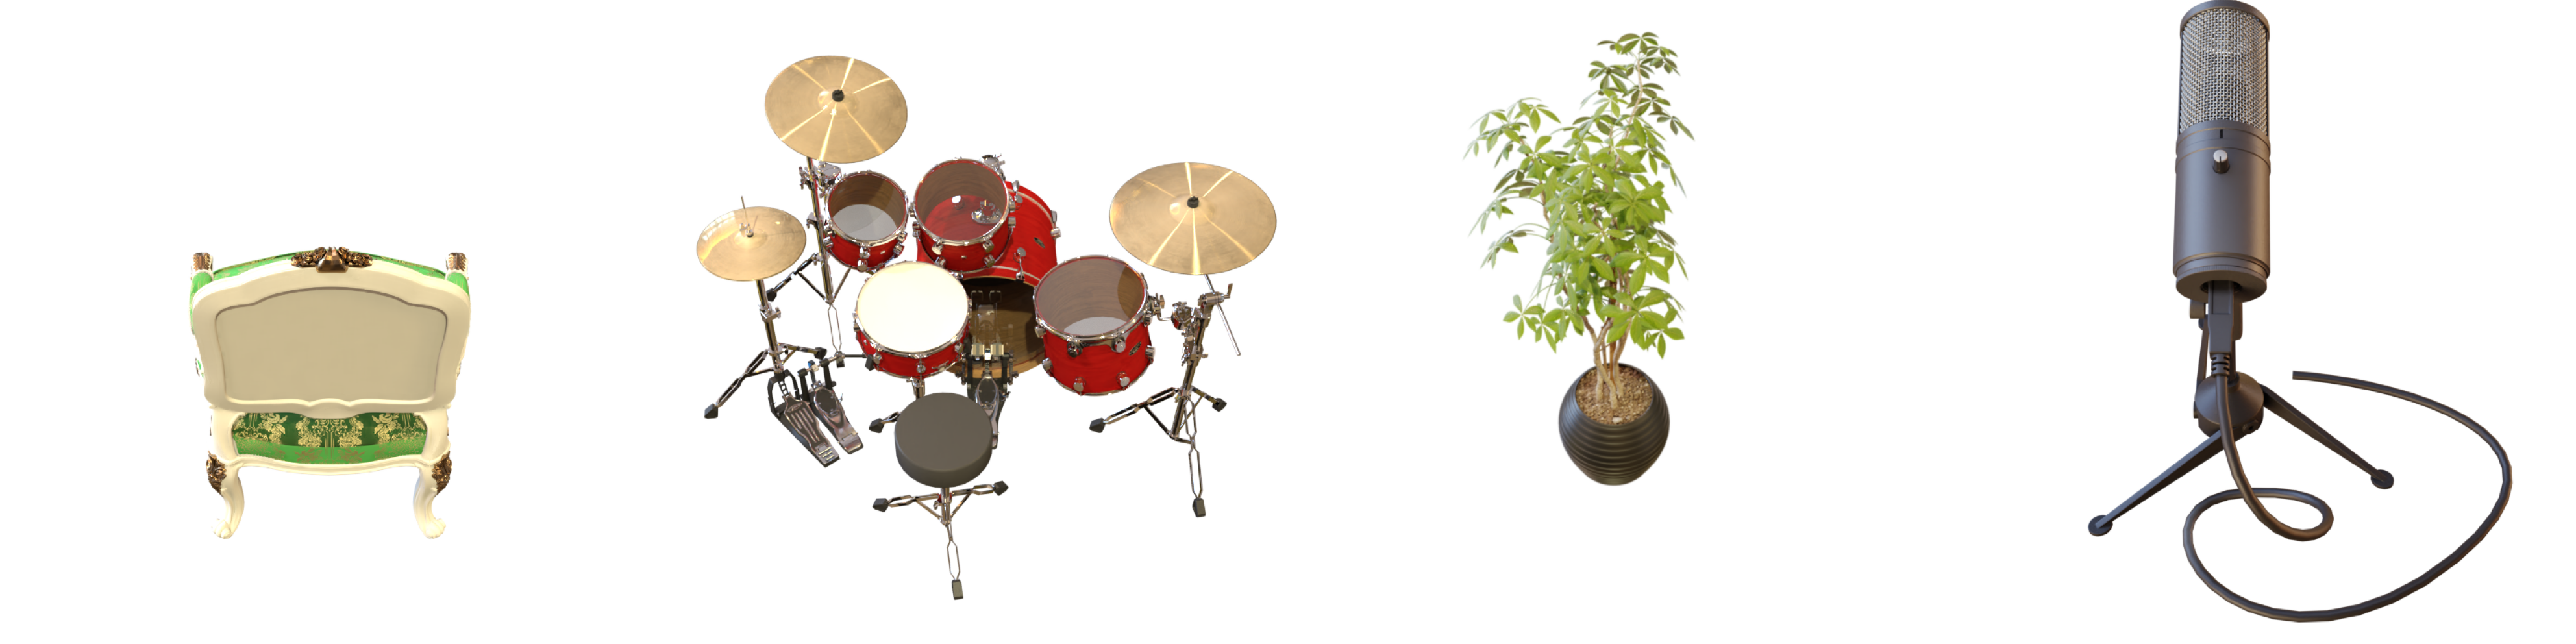}
\caption{Input images from NeRF4 dataset.}
\label{fig:nerf4_dataset}
\end{figure}

\section{Quantitative Results}

\inlinesection{Metrics}

For PSNR and LPIPS, we perform a comparison between the reference image and the generated reference view, which are captured from the same camera pose. This is to ensure a precise evaluation of the reconstruction quality and perceptual similarity in the context of Magic123. The perceptual similarity metric allows us to measure the visual similarity between these two views. Additionally, we utilize CLIP
similarity to calculate the visual similarity between pairs of images by computing their cosine distance in the CLIP encoding space. Specifically, for CLIP-similarity, we compare the reference image with 100 generated views, enabling a thorough assessment of the novel views' resemblance to the reference view.

\inlinesection{Quantitative Results Compared to State-of-the-Art (SOTA)}
To demonstrate the effectiveness of the proposed Magic123, we evaluate its performance on the NeRF4 and RealFusion15 datasets. We conduct a comprehensive and quantitative comparison with multiple baselines for both datasets, as shown in Table~\ref{table:Image-to-3D}. Notably, our method achieves Top-1 performance across all the metrics when compared to previous SOTA approaches. This remarkable performance demonstrates the superiority of Magic123 and its ability to generate high-quality 3D representations.

It is worth noting that the PSNR and LPIPS results demonstrate a significant improvement over the baselines, highlighting the exceptional performance of Magic123 in maintaining both high fidelity in generation and correspondence to the reference frame. 

\input{tables/magic123}

\inlinesection{Detailed per-object quantitative results}
Additionally, we provide the object-wise results of our method compared to the SOTA for both datasets. Magic123 again outperforms the prior works for almost all objects, showing that Magic123 maintains the generalization ability for different objects. 
Results on NeRF dataset are shown in Table.~\ref{tab:nerf}, while results on the Natural images dataset are shown in Table.~\ref{tab:natural}.

% Please add the following required packages to your document preamble:
% \usepackage{booktabs}
% \usepackage{graphicx}
\begin{table}[!htb]
\caption{Object-wise results on NeRF4 dataset.}
\label{tab:nerf}
\resizebox{\textwidth}{!}{%
\begin{tabular}{@{}l|cccc|cccc|cccc@{}}
\toprule
Metrics        & \multicolumn{4}{c|}{\textbf{CLIP-similarity$\uparrow$}}    & \multicolumn{4}{c|}{\textbf{PSNR$\uparrow$}}       & \multicolumn{4}{c}{\textbf{LPIPS$\downarrow$}}      \\ \midrule
Objects        & NeuralLift & 3DFuse & RealFusion & \textbf{Ours} & NeuralLift & 3DFuse & RealFusion & \textbf{Ours}  & NeuralLift & 3DFuse & RealFusion & \textbf{Ours} \\ \midrule
\textit{chair} & 0.59       & 0.57   & 0.36       & \textbf{0.76} & 16.95      & 14.37  & 18.99      & \textbf{30.35} & 0.23       & 0.20   & 0.15       & \textbf{0.02} \\
\textit{drums} & 0.60       & 0.71   & 0.45       & \textbf{0.81} & 10.26      & 7.49   & 13.52      & \textbf{19.49} & 0.47       & 0.47   & 0.31       & \textbf{0.07} \\
\textit{ficus} & 0.38       & 0.47   & 0.28       & \textbf{0.65} & 11.72      & 14.16  & 16.28      & \textbf{21.06} & 0.60       & 0.20   & 0.25       & \textbf{0.05} \\
\textit{mic}   & 0.50       & 0.64   & 0.42       & \textbf{0.81} & 11.27      & 10.56  & 12.68      & \textbf{20.98} & 0.30       & 0.30   & 0.26       & \textbf{0.05} \\ \midrule
\textbf{Average}        & 0.52       & 0.60   & 0.38       & \textbf{0.75} & 12.55      & 11.64  & 15.37      & \textbf{22.97} & 0.40       & 0.29   & 0.24       &\textbf{ 0.05}
\\ \bottomrule
\end{tabular}%
}
\end{table}
% Please add the following required packages to your document preamble:
% \usepackage{booktabs}
% \usepackage{graphicx}
% \usepackage[normalem]{ulem}
% \useunder{\uline}{\ul}{}
\begin{table}[!htb]
\caption{Object-wise results on RealFusion15 dataset.}
\label{tab:natural}
\resizebox{\textwidth}{!}{%
\begin{tabular}{@{}l|cccc|cccc|cccc@{}}
\toprule
Metrics                   & \multicolumn{4}{c|}{\textbf{CLIP-similarity$\uparrow$}}    & \multicolumn{4}{c|}{\textbf{PSNR$\uparrow$}}                & \multicolumn{4}{c}{\textbf{LPIPS$\downarrow$}}               \\ \midrule
Objects                   & NeuralLift & 3DFuse & RealFusion & \textbf{Ours} & NeuralLift & 3DFuse & RealFusion & \textbf{Ours}  & NeuralLift & 3DFuse & RealFusion & \textbf{Ours} \\ \midrule
\textit{banana}           & 0.68       & 0.78   & \textbf{0.83}       & 0.81 & 12.82      & 13.04  & 18.21      & \textbf{18.60} & 0.33       & 0.33   & \textbf{0.12}       & 0.15 \\
\textit{blue bird}             & 0.78       & 0.71   & 0.82       & \textbf{0.87} & 12.40      & 9.73   & 19.53      & \textbf{19.79} & 0.23       & 0.29   & 0.08       & \textbf{0.07} \\
\textit{bird sparrow}     & 0.71       & 0.61   & 0.70       & \textbf{0.82} & 11.01      & 10.96  & \textbf{18.74}      & 17.78 & 0.28       & 0.29   & 0.09       & \textbf{0.07} \\
\textit{cactus}           & 0.73       & 0.76   & 0.69       & \textbf{0.80} & 12.23      & 12.14  & \textbf{18.14}      & 17.73 & 0.26       & 0.25   & \textbf{0.12}       & 0.15 \\
\textit{cake}             & 0.56       & 0.62   & 0.71       & \textbf{0.76} & 10.44      & 10.11  & 17.42      & \textbf{17.64} & 0.75       & 0.44   & \textbf{0.14}       & 0.15 \\
\textit{cat statue}       & 0.63       & 0.59   & 0.64       & \textbf{0.77} & 9.97       & 9.15   & \textbf{18.61}      & 17.88 & 0.38       & 0.43   & 0.12       & \textbf{0.09} \\
\textit{cherry}           & 0.75       & 0.80   & 0.64       & \textbf{0.81} & 10.45      & 11.39  & \textbf{19.40}      & 18.50 & 0.36       & 0.25   & 0.25       & \textbf{0.06} \\
\textit{colorful teapot}  & 0.55       & 0.56   & 0.63       & \textbf{0.64} & 10.17      & 10.94  & 21.34      & \textbf{30.09} & 0.33       & 0.32   & 0.16       & \textbf{0.03} \\
\textit{donut}            & 0.79       & \textbf{0.81}   & 0.63       & 0.74 & 14.00      & 13.17  & 19.87      & \textbf{20.82} & 0.31       & 0.29   & 0.13       & \textbf{0.10} \\
\textit{metal dragon statue}  & 0.61       & 0.61   & 0.66       & \textbf{0.75} & 9.42       & 8.98   & \textbf{17.26}      & 16.40 & 0.39       & 0.43   & \textbf{0.14}       & 0.17 \\
\textit{stone dragon statue}  & 0.63       & 0.65   & 0.65       & \textbf{0.78} & 11.72      & 8.81   & 16.66      & \textbf{17.48} & 0.40       & 0.42   & 0.20       & \textbf{0.16} \\
\textit{fish nemo}        & 0.59       & 0.73   & 0.79       & \textbf{0.89} & 7.95       & 9.56   & 22.88      & \textbf{24.94} & 0.73       & 0.39   & 0.10       & \textbf{0.03} \\
\textit{watercolor horse} & 0.62       & 0.57   & 0.69       & \textbf{0.77} & 8.74       & 6.78   & \textbf{17.08}      & 16.10 & 0.51       & 0.90   & 0.16       & \textbf{0.11} \\
\textit{microphone}       & 0.65       & 0.70   & 0.46       & \textbf{0.82} & 16.42      & 11.77  & 21.85      & \textbf{22.81} & 0.14       & 0.22   & 0.09       & \textbf{0.04} \\
\textit{teddy bear}       & 0.50       & 0.52   & 0.54       & \textbf{0.72} & 8.49       & 8.33   & \textbf{16.10}      & 15.17 & 0.41       & 0.40   & 0.15       & \textbf{0.11} \\ \midrule
\textbf{Average}                   & 0.65       & 0.67   & 0.67       & \textbf{0.78} & 11.08      & 10.32  & 18.87      & \textbf{19.45} & 0.39       & 0.38   & 0.14       & \textbf{0.10} \\
\bottomrule
\end{tabular}%
}
\end{table}

\section{Analysis and Ablation Studies}\label{sec:ablation}
To further show the effectiveness of our method, we provide more quantitative analysis and conduct ablation studies. 

\subsection{Ablation and analysis on the usage of both 2D and 3D priors} 
\inlinesection{3D priors only}
We first turn off the guidance of 2D prior by setting $\lambda_{2D}=0$, such that we only use Zero-1-to-3 \cite{Zero-1-to-3} as a 3D prior.  Furthermore, we study the effects of $\lambda_{3D}$ by performing a grid search and evaluate the image-to-3D reconstruction performance, where  $\lambda_{3D}=5, 10, 20, 40, 60, 80$. Interestingly, we find that Zero-1-to-3 is very robust to the change of $\lambda_{3D}$. \tablabel \ref{tab:ablate_3d} demonstrates that different $\lambda_{3D}$ leads to a consistent quantitative result. We thus simply set $\lambda_{3D}=40$ throughout the experiments since it achieves a slightly better CLIP-similarity score than other values.

\input{tables/ablate_3d}
\input{tables/ablate_2d}

\inlinesection{2D priors only}
We then turn off the 3D prior and study the effect of $\lambda_{2D}$ in the image-to-3D task. As shown in \tablabel \ref{tab:ablate_2d}, with the increase of $\lambda_{2D}$, an increase in CLIP-Similarity and a drop in PSNR are observed. This is because a larger 2D prior weight leads to more imagination, which unfortunately might result in the Janus problem.

\inlinesection{The usage of both 2D and 3D priors and the effects of $\lambda_{div}$}
It is worth noting that using 3D prior only achieves a slighter higher PSNR due to its precise reconstruction but a lower CLIP-similarity because it tends to generate over-simplified geometry.
On the contrary, the 2D prior-based solution achieves a higher CLIP-Similarity but a lower PSNR due to its high imagination capabilities.
Therefore, in our Magic123, we propose to use both 2D and 3D priors. Our novel-view guidance loss is formulated as $\lambda_{div} \mathcal{L}_{2D} + 40\mathcal{L}_{3D}$, where the trade-off parameter $\lambda_{div}$ is used to balance between the geometry exploitation by the 3D prior and the geometry exploration by the 2D prior.
In \figlabel\ref{fig:supp-bothprior} we show that (i) using 2D only prior achieves much better performance in imaging complex scenes such as the drums, but also fails badly in the ficus and microphone examples; (ii) using 3D only prior achieves more precise geometry but fails in complex and uncommon objects (the drums), generating over-simplified back view geometry; (iii) using both 2D and 3D priors achieves a good tradeoff.

\input{figures/supp-bothprior}

% \subsection{Ablation and analysis on the coarse-to-fine two-stage optimization}
% \inlinesection{Coarse stage only}
% Show the results. and study the maximum resolution

% As shown in Fig. {\color{red} xxxx.}, the coarse stage generates low-resolution 3D models with noticeable noise and   low-quality appearance. 

% \inlinesection{Fine stage only}

% Without the coarse stage, the fine stage is trained from scratch, suffering from training instability. As a result, the results using only the fine stage are worse than our method in terms of 3D geometry and quality in Fig. {\color{red} xxxx.}

% \subsection{Ablation and analysis on textural inversion} 
% We ablate textural inversion to show the effect of textural inversion on image-to-3D reconstruction performance. As shown in Fig. {\color{red} xxxx.},  the generated 3D content suffer from view inconsistency issue without textural inversion. For example,  the texture and geometry of the back view are rather inconsistent  with that of  the reference image.

\subsection{Ablation on the resolution}
The ablation study on the choice of resolution is shown in Table.~\ref{tab:ablate_resolution}. We find a trend that the higher the resolution, the better the generation quality. We empirically find that the highest resolution, 256 (requiring 32G memory GPU), gives the best generation quality in terms of quantitative metrics. However, we assume we only have a GPU with 16G memory, therefore we keep using 128 resolution in all our experiments.
% Please add the following required packages to your document preamble:
% \usepackage{booktabs}
% \usepackage{graphicx}
\begin{table}[t]
\centering
\caption{Ablation study on the resolution of the coarse stage for the NeRF4 dataset.}
\label{tab:ablate_resolution}
\resizebox{0.5\textwidth}{!}{%
\begin{tabular}{@{}ccccc@{}}
\toprule
\textbf{Resolution}                & \textbf{32} & \textbf{64} & \textbf{128} & \textbf{256} \\ \midrule
\textbf{CLIP-Similarity$\uparrow$} & 0.7        & 0.8        & 0.8        & \textbf{0.8}         \\
\textbf{PSNR$\uparrow$}            & 20.49       & 22.32       & 22.97       & \textbf{24.22}        \\
\textbf{LPIPS$\downarrow$}           & 0.11        & 0.07        & 0.05        & \textbf{0.03}         \\ \bottomrule
\end{tabular}%
}
\end{table}

\subsection{Ablation on the Noise}
The ablation study on the selection of noise range is shown in Table.~\ref{tab:ablate_noise}. We find the generation quality is not sensitive to the selection of noise range. As we change our noise ranges, the quantitative metrics just have mild changes following the noise range.
% Please add the following required packages to your document preamble:
% \usepackage{booktabs}
% \usepackage{graphicx}
\begin{table}[t]
\centering
\caption{Ablation study on the selection of noise range for the NeRF4 dataset.}
\label{tab:ablate_noise}
\resizebox{0.6\textwidth}{!}{%
\begin{tabular}{@{}ccccccc@{}}
\toprule
\textbf{Noise} & \textbf{{[}0.02, 0.6{]}} & \textbf{{[}0.1,0.6{]}} 
&\textbf{{[}0.2,0.6{]}}
& \textbf{{[}0.2,0.8{]}} & \textbf{{[}0.2,0.98{]}} & \textbf{{[}0.4,0.6{]}} \\ \midrule
\textbf{CLIP-Similarity$\uparrow$} & 0.8  & 0.8  & 0.8& 0.8  & 0.8  & 0.8  \\
\textbf{PSNR$\uparrow$}            & 24.1 & 22.5 & 23.0 & 24.0 & 23.6 & 23.7 \\
\textbf{LPIPS$\downarrow$}           & 0.04  & 0.05  & 0.05 & 0.04  & 0.04  & 0.04  \\ \bottomrule
\end{tabular}%
}
\end{table}

\section{Implementation Details}
We build our Magic123 upon the popular open-source repository, Stable DreamFusion~\cite{stable-dreamfusion}.
We train our Magic123 on an NVIDIA 16G V100 GPUs for 5000 iterations for the coarse stage and 10000 iterations for the fine stage. We set the learning rate to $1e-3$ with Adam optimizer without learning rate decay. We adopt the Stable Diffusion~\cite{DiffusionModels} model of V1.5. For the 3D prior, we adopt the pretrained Zero-1-to-3 \cite{Zero-1-to-3} that was finetuned the least (105,000 iterations).

% Following Magic3D \cite{Magic3D}, we adopt Instant-NGP \cite{InstantNGP} as the 3D representation in the coarse stage,  where we use MLPs to predict rendered images from color and volume density. In the fine stage, we use the marching cube algorithm to convert the NeRF representation into DMTet~\cite{DMTet} representation, then we utilize differentiable rendering to optimize the texture and geometry at the same time.
% 

\section{Additional qualitative results}\label{sec:supp_qualitative}
We provide qualitative comparisons with additional prior works including RealFusion \cite{RealFusion} ($4^{th} col$),  NeuralLift~\cite{NeuralLift} ($5^{th}$ col),  3DFuse~\cite{3DFuse} ($6^{th}$ col), Point-E \cite{PointE} ($7^{th}$ col), and Shap-E \cite{ShapeE}($8^{th}$ col) for generating 3D object from a single unposed image (the leftmost column) in \figlabel\ref{fig:supp-sota1}. 

\input{figures/supp-sota1}
